# Supplementary material for: Information Anxiety in Large Language Models
Source: arXiv:2411.10813 source file (2024-11-16)
Supplement: Supplementary file 1 [file additional_information_methods_paraphrases_capital.tex]

\begin{table}[h!]
\setlength{\tabcolsep}{2pt} % Adjusting column separation
 % Reducing cell padding
\resizebox{\textwidth}{!}{%
\begin{tabular}{p{1.2in}@{\hspace{4em}}p{5.2in}}
\\
\textbf{\texttt{capital}} & 
    \begin{tabular}{l}
        What is the \format{capital} of <MASK>?\\
        What is the \format{primary city} in <MASK>?\\
        Which \format{urban center} holds a \format{central role} in <MASK>?\\
        Which city \format{houses the main government} of <MASK>?\\
        What city is the \format{main administrative center} of <MASK>?\\
        What \format{urban area} holds the \format{capital status} of <MASK>?\\
        Which city is the \format{political focal point} of <MASK>?\\
        Which city is the \format{primary seat of authority} for <MASK>?\\
        What is the \format{principal city} of <MASK>?\\
        What is the \format{chief city} of <MASK>?\\
    \end{tabular}\\
\end{tabular}
}
\end{table}
