# Supplementary material for: Information Anxiety in Large Language Models
Source: arXiv:2411.10813 source file (2024-11-16)
Supplement: Supplementary file 2 [file additional_information_methods_paraphrases_genre.tex]

\begin{table}[h!]
\setlength{\tabcolsep}{2pt} % Adjusting column separation
 % Reducing cell padding
\resizebox{\textwidth}{!}{%
\begin{tabular}{p{1.2in}@{\hspace{4em}}p{5.2in}}
\\
\textbf{\texttt{genre}} & \begin{tabular}{l}
        What \format{category} does <MASK> belong to?\\
        What \format{kind of classification} does <MASK> fall under?\\
        What \format{type} does <MASK> fall under?\\
        What \format{group} does <MASK> fall under?\\
        What \format{kind} does <MASK> fall under?\\
        What \format{class} does <MASK> fall under?\\
        What \format{style} can <MASK> be categorized into?\\
        Which \format{division} does <MASK> come under?\\
        In what \format{bracket} does <MASK> reside?\\
        What \format{domain} does  <MASK> fit within?\\
\end{tabular}\\
\bottomrule
\end{tabular}
}
\end{table}
