# Supplementary material for: Information Anxiety in Large Language Models
Source: arXiv:2411.10813 source file (2024-11-16)
Supplement: Supplementary file 3 [file additional_information_methods_paraphrases_occupation.tex]

\begin{table}[h!]
\setlength{\tabcolsep}{2pt} % Adjusting column separation
 % Reducing cell padding
\resizebox{\textwidth}{!}{%
\begin{tabular}{p{1.2in}@{\hspace{4em}}p{5.2in}}
\\
\textbf{\texttt{occupation}} & \begin{tabular}{l}
    What does <MASK> do for a \format{living}?\\
    What is <MASK>'s \format{occupation}?\\
    What is <MASK>'s \format{profession}?\\
    What is <MASK>'s \format{line of work}?\\
    What \format{job role} is <MASK> engaged in?\\
    What \format{career path} has <MASK> chosen?\\
    What \format{field of employment} is <MASK> part of?\\
    What is <MASK>'s source of \format{professional engagement}?\\
    What is <MASK>'s \format{vocational pursuit}?\\
    What \format{field of work} is <MASK> engaged in?\\
\end{tabular}\\
\\
\end{tabular}
}
\end{table}
