# Supplementary material for: Information Anxiety in Large Language Models
Source: arXiv:2411.10813 source file (2024-11-16)
Supplement: Supplementary file 4 [file additional_information_methods_paraphrases_religion.tex]

\begin{table}[h!]
\setlength{\tabcolsep}{2pt} % Adjusting column separation
 % Reducing cell padding
\resizebox{\textwidth}{!}{%
\begin{tabular}{p{1.2in}@{\hspace{4em}}p{5.2in}}
\\
\textbf{\texttt{religion}} & \begin{tabular}{l}

        What is the \format{religion} of <MASK>?\\
        What \format{faith} does <MASK> follow?\\
        What is the \format{religious affiliation} of <MASK>?\\
        Which \format{religious doctrine} does <MASK> subscribe to?\\
        What \format{theology} is <MASK> aligned with?\\
        What is the \format{religious identity} of <MASK>?\\
        What \format{belief system} does <MASK> ascribe to?\\
        What \format{religious school of thought} does <MASK> follow?\\
        What is <MASK>'s \format{spirituality}?\\
        What is the \format{religious allegiance} of <MASK>?\\

\end{tabular}\\
\end{tabular}
}
\end{table}
