# Supplementary material for: Information Anxiety in Large Language Models
Source: arXiv:2411.10813 source file (2024-11-16)
Supplement: Supplementary file 5 [file additional_information_methods_paraphrases_screenwriter.tex]

\begin{table}[h!]
\setlength{\tabcolsep}{2pt} % Adjusting column separation
 % Reducing cell padding
\resizebox{\textwidth}{!}{%
\begin{tabular}{p{1.2in}@{\hspace{4em}}p{5.2in}}
\\
\\
\textbf{\texttt{screenwriter}} & \begin{tabular}{l}
        Who was the \format{screenwriter} for <MASK>?\\
        Who \format{wrote the screenplay} for <MASK>?\\
        Who was the \format{scribe of the screenplay} in <MASK>?\\
        Who took on the \format{role of crafting} <MASK>'s \format{script}?\\
        Who was responsible for \format{composing the screenplay} of <MASK>?\\
        Who was the \format{wordsmith behind the screenplay} of <MASK>?\\
        Who \format{penned the script} for <MASK>?\\
        Who \format{authored the screenplay} of <MASK>?\\
        Who was the primary influencer in shaping <MASK>'s \format{screenplay composition}?\\
        Who \format{scripted} <MASK>'s story?\\
\end{tabular}\\
\\
\end{tabular}
}
\end{table}
