# Supplementary material for: Information Anxiety in Large Language Models
Source: arXiv:2411.10813 source file (2024-11-16)
Supplement: Supplementary file 6 [file additional_information_methods_paraphrases_sport.tex]

\begin{table}[h!]
\setlength{\tabcolsep}{2pt} % Adjusting column separation
 % Reducing cell padding
\resizebox{\textwidth}{!}{%
\begin{tabular}{p{1.2in}@{\hspace{4em}}p{5.2in}}
\\
\textbf{\texttt{sport}} & \begin{tabular}{l}
        What \format{sport} does <MASK> play?\\
        What \format{athletic activity} does <MASK> participate in?\\
        What \format{game} does <MASK> compete in?\\
        What \format{field of sports} is <MASK> involved with?\\
        Which \format{athletic endeavour} does <MASK> pursue?\\
        What \format{physical activity} does <MASK> perform as a sport?\\
        What \format{recreational sport} does <MASK> enjoy?\\
        What \format{sport} does <MASK> enjoy playing?\\
        What \format{professional sport} does <MASK> play?\\
        What \format{game} does <MASK> actively participate in?\\
\end{tabular}\\
\bottomrule
\end{tabular}
}
\end{table}
