# Supplementary material for: Information Anxiety in Large Language Models
Source: arXiv:2411.10813 source file (2024-11-16)
Supplement: Supplementary file 7 [file supplementary.tex]

\documentclass[10pt]{wlscirep}
\usepackage[utf8]{inputenc}
\usepackage[T1]{fontenc}
\usepackage{float}
\usepackage{longtable}
\usepackage{todonotes}
\usepackage{booktabs}
\usepackage{array}
\usepackage{graphicx}
\pdfobjcompresslevel=0

%%%%%%%%%%%%%%%%%%%%%  BLOCK TITLE %%%%%%%%%%%%%%%%%%%%%%%%
% \title{Information Anxiety in Large Language Models}

% %: Analysing the Effect of Popularity on the Internal LLM Structures.}
% % \title{Do LLMs Have Stage Fright?: Analysing the Effect of Popularity on the Internal LLM Structures.}
% \author[1]{Prasoon Bajpai}
% \author[2,3,*]{Tanmoy Chakraborty}
% \affil[1]{Department of Mathematics, Indian Institute of Technology, Delhi, New Delhi, India}
% \affil[2]{Department of Electrical Engineering, Indian Institute of Technology, Delhi, New Delhi, India}
% \affil[3]{Yardi School of Artificial Intelligence, Indian Institute of Technology, Delhi, New Delhi, India}
% \affil[*]{Corresponding author: tanchak@iitd.ac.in}
% %\affil[2]{subhabrata.dutta@tu-darmstadt.de}
%%%%%%%%%%%%%%%%%%%%%%%%%%%%%%%%%%%%%%%%%%%%%%%%%%%%%%%%%%%%
%\keywords{Keyword1, Keyword2, Keyword3}

% \input{sections/abstract}
\begin{document}
\flushbottom
% \maketitle
% * <john.hammersley@gmail.com> 2015-02-09T12:07:31.197Z:
%
%  Click the title above to edit the author's information and abstract
%
% \thispagestyle{empty}

% \input{sections/introduction.tex}
% \input{sections/results.tex}
% \input{sections/discussion.tex}
% \input{sections/methods.tex}
% \input{sections/references.tex}
% \input{sections/author_contributions_statement}
% \newpage
% \input{sections/additional_information}
\input{sections/supplementary_information}

\end{document}
